# Supplementary material for: Decoupled interband pairing in a bilayer iron-based superconductor evidenced by ultrahigh-resolution ARPES
Source: arXiv:2601.07380 source file (2026-01-12)
Supplement: Supplementary file 1 [file SM.pdf]

# Decoupled interband pairing in a bilayer iron-based superconductor evidenced by ultrahigh-resolution angle-resolved photoemission spectroscopy: Supplemental Material

Shichong Wang,[1,2] Yuanyuan Yang,[1] Yang Li,[2,3] Wenshan Hong,[2] Huaxun Li,[4] Shaofeng Duan,[2,1] Lingxiao Gu,[1,2] Haoran Liu,[1,2] Jiongyu Huang,[1,2] Jianzhe Liu,[1,2] Dong Qian,[1,5,6] Guanghan Cao,[4,5] Huiqian Luo,[2] and Wentao Zhang[2,1,*]

[1]*Key Laboratory of Artificial Structures and Quantum Control (Ministry of Education), School of Physics and Astronomy, Shanghai Jiao Tong University, Shanghai 200240, China*

[2]*Beijing National Laboratory for Condensed Matter Physics, Institute of Physics, Chinese Academy of Sciences, Beijing 100190, China*

[3]*School of Physical Sciences, University of Chinese Academy of Sciences, Beijing 100190, China*

[4]*School of Physics, Zhejiang University, Hangzhou 310058, China*

[5]*Collaborative Innovation Center of Advanced Microstructures, Nanjing University, Nanjing 210093, China*

[6]*Tsung-Dao Lee Institute, Shanghai Jiao Tong University, Shanghai 200240, China*

## Abstract

This Supplemental Material includes five additional discussions, five additional figures, and one supplementary data table.

[*] wentaozhang@iphy.ac.cn

## I. METHODS

High-quality single crystals of $KCa_2Fe_4As_4F_2$ and $CsCa_2Fe_4As_4F_2$ were synthesized via flux method [S1–4]. Bulk superconductivity was confirmed by transport measurements, revealing sharp transitions at $T_c$ = 33.5 K (K12442) and 30 K (Cs12442). Ultrahigh-resolution ARPES was performed with a 7 eV vacuum ultraviolet laser featuring an amplified repetition rate of 2 GHz to minimize space charge effects. This setup achieved an exceptional energy resolution of 0.26 meV at high count rates [S5], thereby enabling the precise and efficient tracking of the temperature-dependent energy gap [S6]. The laser spot size on the sample is approximately 35 $\mu$m. The probe laser is operating at a repetition rate of 2 GHz to reduce the space charge effect while maintaining high photon flux. Samples were cleaved in situ under ultra-high vacuum ($< 3 \times 10^{-11}$ torr). During the temperature-dependent measurements, the beam spot on the sample was stablized with an accuracy better than 1 $\mu$m using a sample-position auto correction system [S7]. Leveraging the low work function of approximately 3 eV in this sample, we utilized a 7 eV laser to achieve ultrahigh-resolution measurements of the electronic states near the M point in K12442.

## II. CONCLUSIVE EXPERIMENTAL OBSERVATION

The observation of dual superconducting transitions is an intrinsic property of the bulk material, ruling out explanations based on surface termination heterogeneity or bulk-surface discrepancies. This conclusion is firmly supported by the following experimental evidence: (i) identical spectral features, including consistent multi-gap characteristics with gap sizes agreeing with prior studies [S8, 9], are observed across multiple cleaved surfaces (with STM-dominant termination [S8]); (ii) the clear resolution of two distinct Fermi surfaces, corresponding to bilayer-split bands from inter bilayer hopping within the double $Fe_2As_2$ layers, provides direct evidence of electronic splitting without mixed termination signals; (iii) analysis of the Fermi surface sizes of the $\beta_1$ and $\beta_2$ bands in K12442 further corroborates the bilayer splitting scenario, as the $\beta_1$ band—though possessing a smaller energy gap—does not exhibit the larger hole pocket expected from additional hole doping, which would occur if it were a surface state due to potassium loss; (iv) this interpretation is strengthened by contrasting these results with those from Cs12442, where, despite the greater tendency of Cs atoms to escape from the cleaved surface and potentially create multiple terminations [S10], all Cs samples exhibit only a single transition at $T_c$ = 30 K with no evidence of a

surface-related transition at lower temperature.

## III. EDCS ON THE FERMI SURFACE SHEETS

Accurate determination of the Fermi momentum ($k_F$) is a prerequisite for reliable energy gap extraction. As shown in Fig. S3(a), the spectrum divided by the Fermi-Dirac distribution clearly demonstrates the transition of the energy gap in K12442, allowing for the extraction of the Fermi momentum $k_F$ from the Fermi crossing above $T_c$. We observe that the energy gaps of the $\alpha$ and $\beta_1$ bands are nearly closed between 14 K to 24 K,whereas those of the $\gamma$ and the $\beta_2$ bands persist up to $T_{\mathrm{c}}$ = 33.5 K. This asynchronous gap closure provides direct evidence for two distinct critical temperatures within the split bands. Additionally, since the $k_F$ values of the $\beta_1$ and $\beta_2$ bands show negligible difference above $T_c$, we omit separate EDC analyses for these bands in the main text.

Figures S3(a) and (c) display the temperature-dependent photoemission spectra of K12442 and Cs12442 divided by the Fermi-Dirac distribution (FD) function. Distinct Bogoliubov quasiparticle peaks are observed above the Fermi level ($E_F$), providing direct evidence of particle-hole symmetry. The EDCs of different bands, as discussed in main text, were selected to be divided by the Fermi-Dirac distribution function, and compared them with the symmetrized EDCs and raw data. To resolve the Bogoliubov peaks above $E_F$, the analysis focuses on temperatures slightly below $T_c$, as electrons occupy states above the Fermi level. The consistency between the FD-divided peaks and the symmetrized data confirms the particle-hole symmetry and validates the symmetrization procedure employed in the main text.

The absence of a pseudogap in the hole pockets near the Γ point was confirmed by temperature-dependent ARPES experiments above $T_c$. To further clarify this, we extracted the energy gap of the $\beta$ band and the intensity near the Fermi level in K12442 above the superconducting transition temperature ($T_c = 33.5$ K). The symmetrized EDCs of the $\beta$ band collapse into a single peak above $T_c$ (Fig. S4(a)), indicating the complete closure of the energy gap. Furthermore, the spectral intensity remains nearly constant between 33.5 K and 70 K (Fig. S4(b)), showing no indication of a pseudogap . A similar behavior was observed for the other energy bands near the Γ point and in Cs samples, as detailed in Fig. 2 of the main text.

## IV. BCS GAP FITTING PROCEDURE

To determine the superconducting transition temperature, we analyzed experimental temperature-dependent energy gap data through numerical fitting procedures grounded in the BCS self-consistent equation [S11]

$$G(\Delta) = \ln\frac{T}{T_\mathrm{c}} + \pi k_\mathrm{B}T\sum_{\epsilon_n}\left[\frac{1}{|\epsilon_n|} - \frac{1}{\sqrt{\epsilon_n^2+\Delta^2}}\right], \quad \text{(S16)}$$

by introducing $\epsilon_n = 2\pi k_\mathrm{B}T(n-\frac{1}{2})$ ($n$ is a positive integer), we obtain the numerical solution for the BCS energy gap as a function of temperature. The numerical calculation begins with an initial guess for superconducting transition temperature $T_\mathrm{c}$ and energy gap size $\Delta(0)$, and iterates to derive a temperature-dependent energy gap equation, continuing until the discrepancy between the calculated results and experimental data falls within an acceptable error. Such fitting procedure yields errors in $T_\mathrm{c}$ of less than 1.5 K, as shown in TABLE I. The fitted transition temperatures indicate a dual transition regime in K12442 but a single transition $T_\mathrm{c} = T_\mathrm{c,bulk} \sim$ 30 K in Cs12442. For various bands in K12442, an earlier transion temperature $T_\mathrm{c}^* \sim$ 22 K is reasonably fitted from the temperature-dependent energy gap data for the $\alpha$, $\beta_1$ and $\varepsilon$ bands, whereas other bands follow the bulk transition at $T_\mathrm{c} \sim$ 33.5 K, demonstrating consistency with Figs. 2 and 3 in the main text.

## V. NUMERICAL SIMULATION OF TWO-BAND MODEL

A two-band weak-coupling model based on Eilenberger theory was employed to explain the bandgap transition phenomenon in multi-band superconductors [S12, 13]. Here, the formula and the numerical solution presented in the main text will be discussed in more detail.

Starting with the Eilenberger quasiclassical version of Gor'kov's theory [S14], a concise representation of the anisotropic Fermi surface is given by

$$\boldsymbol{v}\boldsymbol{\Pi}f = 2\Delta g/\hbar - 2\omega f, \quad \text{(S1)}$$

$$-\boldsymbol{v}\boldsymbol{\Pi}^* f^+ = 2\Delta^* g/\hbar - 2\omega f^+, \quad \text{(S2)}$$

$$g^2 = 1 - ff^+, \quad \text{(S3)}$$

$$\Delta(\boldsymbol{r},\boldsymbol{v}) = 2\pi T N(0)\sum_{\omega}^{\omega_\mathrm{D}} \langle V(\boldsymbol{v},\boldsymbol{v}')f(\boldsymbol{v}',\boldsymbol{r},\omega)\rangle_{\boldsymbol{v}'}\,. \quad \text{(S4)}$$

In these equations, $\Delta(\boldsymbol{r})$ is the gap function at $\mathbf{k}_F$ values or different Fermi velocities $\boldsymbol{v}$. The operator $\mathbf{\Pi}$ is defined as $\nabla + 2\pi i\mathbf{A}/\phi_0$, where $\phi_0$ is the flux quantum. The functions $f$, $g$, and $f^+$ correspond to the Eilenberger Green function. $N(0)$ denotes the density of states at the Fermi energy for each spin. $\omega = \omega_m$ represents the Matsubara frequencies, defined as $\hbar\omega = \pi T(2m+1)$, where $m$ is a positive integer, and $\omega_{\mathrm{D}}$ denotes the Debye frequency. The average intensity at the Fermi surface is defined as

$$\langle X \rangle = \int \frac{d^2\mathbf{k}_F}{(2\pi)^3 \hbar N(0)|\boldsymbol{v}|} X. \tag{S5}$$

Considering the two-band model, the energy gap at different Fermi momentum $\mathbf{k}_F$ can be written by

$$\Delta(k) = \Delta_{1,2}, \quad k \in F_{1,2}, \tag{S6}$$

where $F_1$ and $F_2$ represent two sets of Fermi surface sheets. Since only two state densities $N_1$ and $N_2$ are considered, the average weight on each Fermi surface sheet is written by

$$\langle X \rangle = (X_1 N_1 + X_2 N_2)/N(0) = n_1 X_1 + n_2 X_2, \tag{S7}$$

where $n_{1,2} = N_{1,2}/N(0)$ with $n_1 + n_2 = 1$. This analysis assumes the absence of electric and magnetic fields, implying that $\mathbf{\Pi} = 0$. Under these conditions, the Eilenberger equations reduce to

$$f_\nu = \frac{\Delta_\nu}{\beta_\nu}, \quad g_\nu = \frac{\hbar\omega}{\beta_\nu}, \quad \beta_\nu^2 = \Delta_\nu^2 + \hbar^2\omega^2, \tag{S8}$$

where $\nu = 1, 2$ represents the band index and $\beta_\nu$ depends on the position of the Fermi momentum $\mathbf{k}_F$.

In the above case, the energy gap equation Eq. (S4) for a simple two-band system can be written by

$$\Delta_\nu = 2\pi T \sum_{\mu=1,2} \lambda_{\nu\mu} f_\mu = \sum_\mu \lambda_{\nu\mu} \Delta_\mu \sum_\omega^{\omega_{\mathrm{D}}} \frac{2\pi T}{\beta_\mu}, \tag{S9}$$

where $\lambda_{\nu\mu}$ denotes the band interaction and should be proportional to the density of states, i.e., $\lambda_{\nu\mu} = n_\mu N(0) V_{\nu\mu}$. $V_{\nu\mu}$ represents the effective coupling potential in the two band system.

For the limit where $T \to T_{\mathrm{c}}$, with $\Delta \to 0$ and $\beta \to \hbar\omega$. the summation term of Eq. (S9) gives

$$S = \sum_\omega^{\omega_D} \frac{2\pi T}{\hbar\omega} = \ln \frac{2\hbar\omega_D}{T_{\mathrm{c}} \pi e^{-\gamma}} \approx \ln \frac{2\hbar\omega_D}{1.76 T_{\mathrm{c}}}. \tag{S10}$$

The constant $\pi e^{-\gamma} \approx 1.76$ ($\gamma$: Euler constant) is characteristic of BCS superconductors and is independent of the material.

By substituting $S$ into Eq. (S9), the relationship between $S$ and $\lambda$ is obtained,

$$\Delta_1 = S\left(\lambda_{11}\Delta_1 + \lambda_{12}\Delta_2\right), \ \Delta_2 = S\left(\lambda_{21}\Delta_1 + \lambda_{22}\Delta_2\right). \tag{S11}$$

To ensure a non-trivial solution for this system of equations,

$$S = \frac{\lambda_{11} + \lambda_{22} - \sqrt{(\lambda_{11} - \lambda_{22})^2 + 4\lambda_{12}\lambda_{21}}}{2(\lambda_{11}\lambda_{22} - \lambda_{12}\lambda_{21})}. \tag{S12}$$

For temperature far away from the $T_c$,

$$S = \sum_{\omega}^{\omega_{\mathrm{D}}} \frac{2\pi T}{\hbar\omega} + \ln\frac{T}{T_{\mathrm{c}}}. \tag{S13}$$

The temperature correction term, $\ln(T/T_{\mathrm{c}})$, can be calculated by converting the discrete summation involving the energy gap in Eq. (S9) into an integral form. In our numerical calculations, $S$ was evaluated from Eq. (S12) for different coupling coefficients $\lambda_{\nu\mu}$. Now the Eq. (S9) is written as

$$\Delta_\nu = \sum_{\mu} \lambda_{\nu\mu}\Delta_\mu \left[\sum_{\omega}^{\infty}\left(\frac{2\pi T}{\beta_\mu} - \frac{2\pi T}{\hbar\omega}\right) + S - \ln\frac{T}{T_{\mathrm{c}}}\right]. \tag{S14}$$

By treating the Matsubara frequencies $\omega = \omega_m$ as integers, the equation of energy gap gives

$$\Delta_\nu = \sum_{\mu=1,2} \lambda_{\nu\mu}\Delta_\mu \left[\left(S + \ln\frac{T}{T_{\mathrm{c}}}\right) - \sum_{m=0}^{\infty}\left(\frac{1}{m+1/2} - \frac{1}{\sqrt{\left(\frac{\Delta\nu}{2\pi T}\right)^2 + (m+1/2)^2}}\right)\right]. \tag{S15}$$

Building on the above equation and chosen coupling coefficients, iterative calculations yield the functional dependence of the energy gap $\Delta_\nu$ on temperature $T$. In the numerically calculated results presented in Fig. 4 of the main text, the summation is truncated at 500 terms—a cutoff confirmed to sufficiently capture the temperature-dependent energy gap with convergence accuracy.

TABLE I. Summary of the transition temperatures $T_c$ and zero-temperature energy gaps $\Delta(0)$ for all resolvable bands in K12442 and Cs12442. Values are derived from BCS fits to the temperature-dependent experimental data. Uncertainties in $\Delta(0)$ are estimated to be less than 0.1 meV.

| | Band index | $\Delta(0)$ (meV) | $T_c$ (K) |
|---|---|---|---|
| K12442 | $\alpha$ | 5.0 | 22.4 $\pm$ 0.4 |
| | $\beta_1$ | 4.3 | 23.0 $\pm$ 0.8 |
| | $\beta_2$ | 8.3 | 33.4 $\pm$ 1.4 |
| | $\gamma$ | 2.3 | 34.4 $\pm$ 0.2 |
| | $\varepsilon$ | 4.3 | 20.5 $\pm$ 0.1 |
| Cs12442 | $\alpha$ | 7.9 | 31.9 $\pm$ 0.3 |
| | $\beta$ | 7.3 | 31.8 $\pm$ 0.3 |
| | $\gamma_1$ | 2.1 | 31.6 $\pm$ 0.9 |
| | $\gamma_2$ | 1.8 | 30.5 $\pm$ 0.6 |

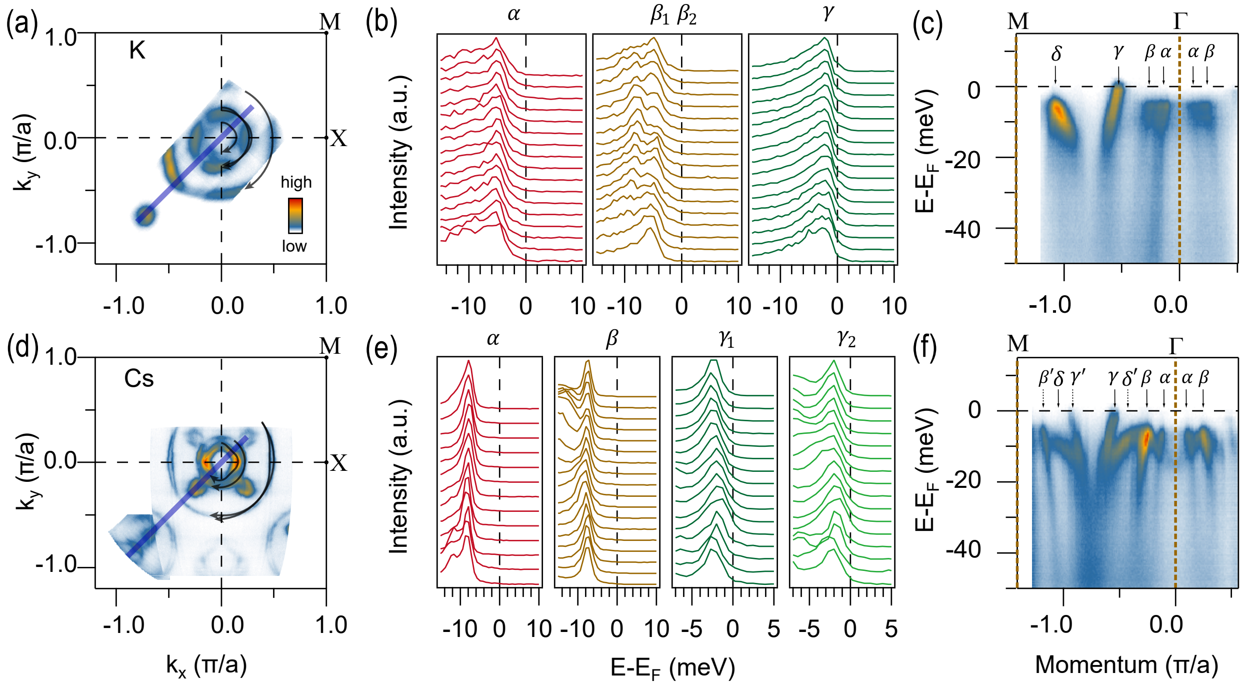


Fig. S1. Raw data for K12442 (upper panel) and Cs12442 (lower panel). (a) Photoemission contour for K12442 at a binding energy of 10 meV. The black arrows indicate the momentum measurement of different Fermi surface sheets, and the blue line denotes the cut direction from Γ(0, 0) to M($\pi$, $\pi$). (b) Raw EDCs for Fig. 1(b) in the main text, showing the energy gap evolution along the different Fermi surface sheets of K12442. (c) Band structures along Γ-M in K12442, with the cut direction indicated by the blue solid line in (a). Black arrows denote different energy bands, and dashed arrows indicate folded bands. (d-f) Corresponding measurements for Cs12442.

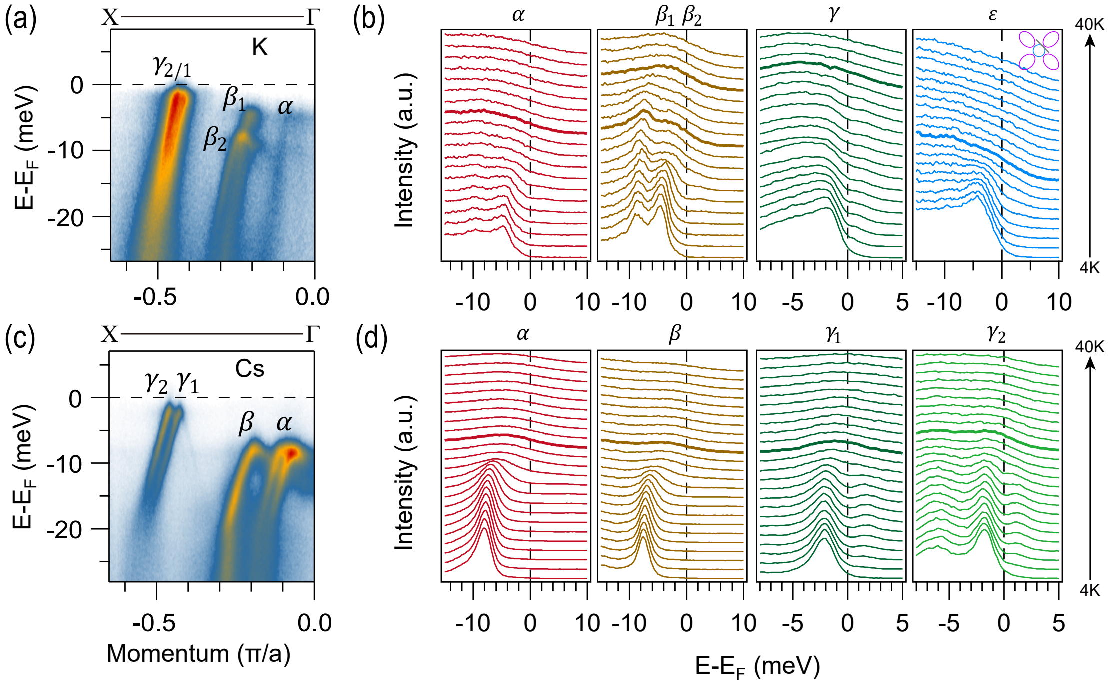


Fig. S2. Raw EDCs from temperature-dependent experiments of K12442 (upper panel) and Cs12442 (lower panel). (a) Photoemission spectrum of K12442 measured at 4 K, with band indices marked; the corresponding spectrum for Cs12442 is shown in (c). (b) Raw EDCs of K12442, corresponding to the symmetrized results in Figs. 2(d) and 3(b) of the main text. (d) Raw EDCs of Cs12442, corresponding to Fig. 2(h) of the main text (Cs12442). The bold lines in (b) and (d) indicate EDCs taken at the transition temperature..

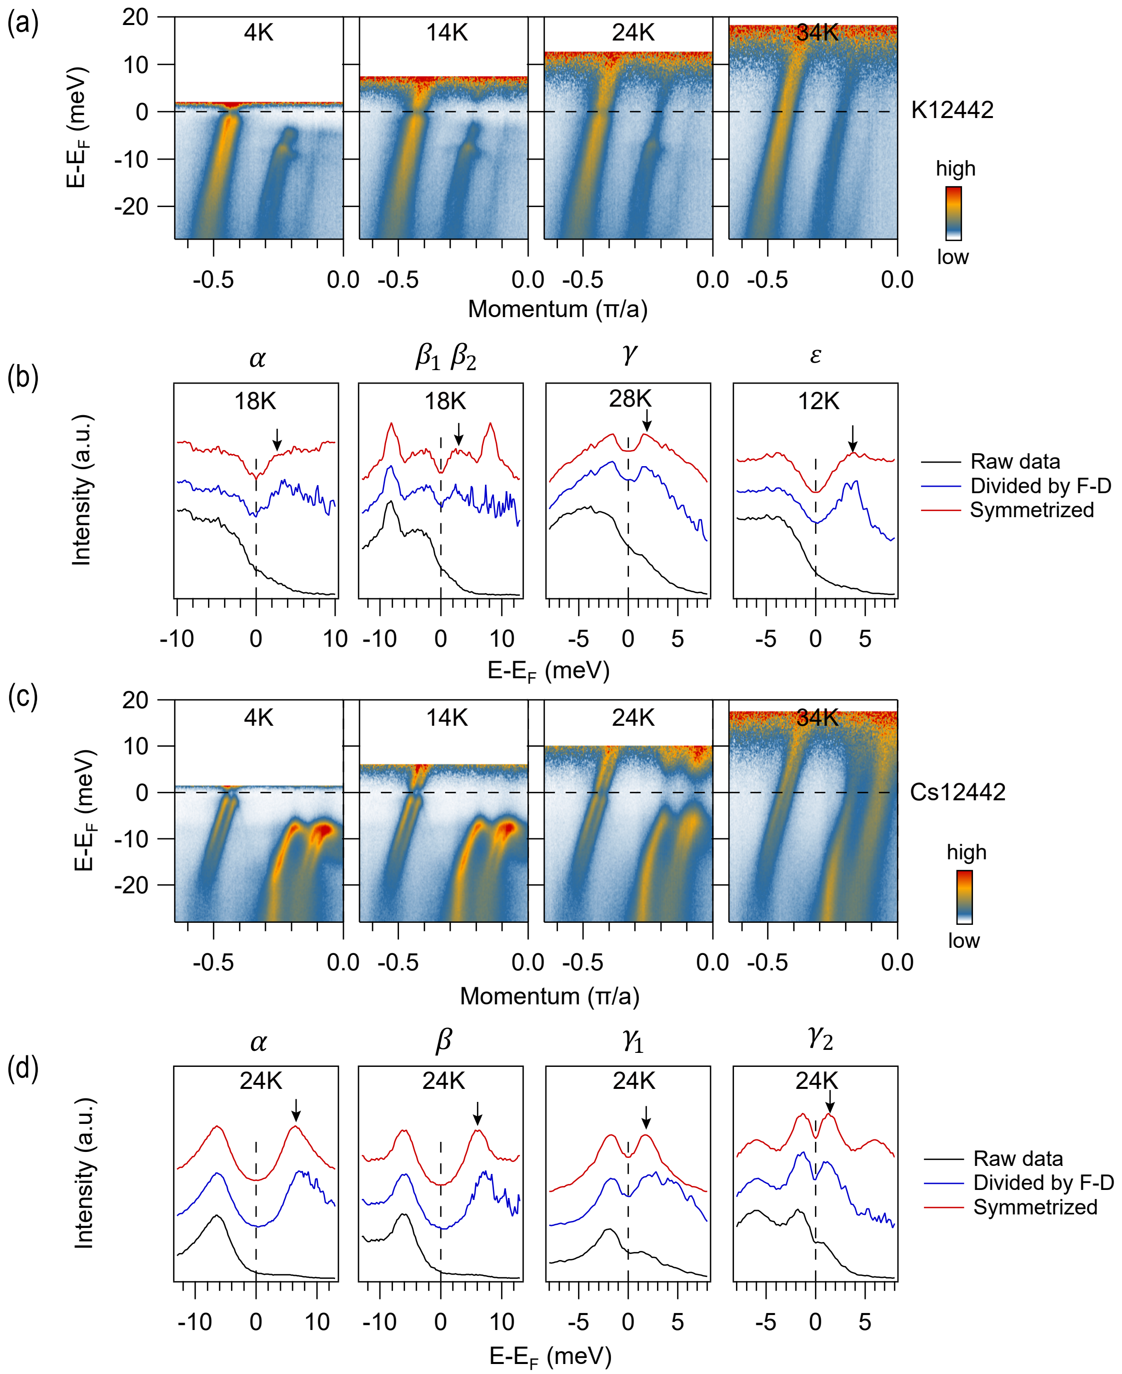


Fig. S3. Temperature-dependent photoemission spectrum and EDCs divided by the Fermi-Dirac distribution (FD) in K12442 and Cs12442. (a) FD-divided spectrum of K12442 measured at 4 K, 14 K, 24 K, and 34 K. (b) Comparison of the FD-divided EDCs (taken below $T_c$) with raw data and symmetrized EDCs. Black arrows indicate the Bogoliubov quasiparticle peaks. (c)-(d) Corresponding measurements for Cs12442.

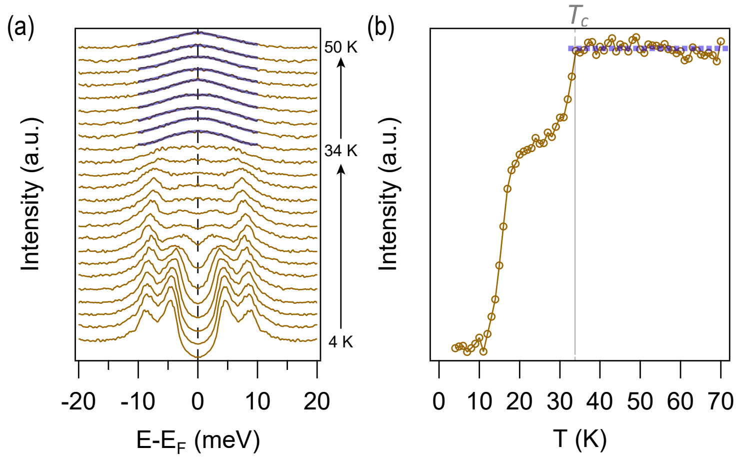


Fig. S4. Temperature evolution of the $\beta$ band in K12442. (a) Symmetrized EDCs for the $\beta$ band from 4 K to 50 K. Blue solid curves are fits to the data above above $T_c$. (b) Temperature-dependent intensity integrated near the Fermi energy for $\beta$ band up to 70 K. The blue dashed line serves as a guideline indicating the intensity remains constant above $T_c$.

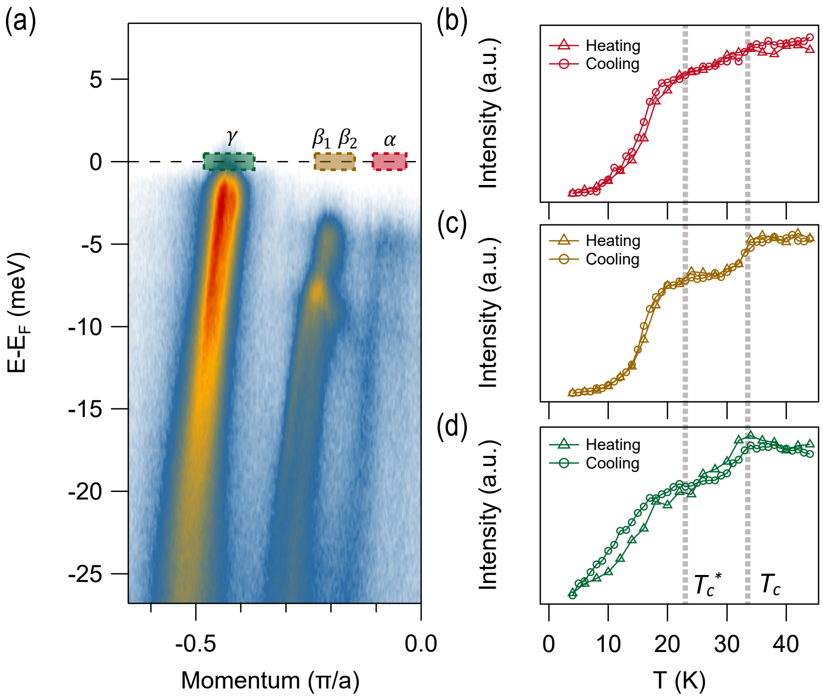


Fig. S5. Comparison between heating and cooling cycles in K12442. (a) Low-temperature photoemission spectrum. Colored markers indicate the momentum integration ranges for the three bands, with the energy range being $E_F \pm$ 0.5 meV. (b)-(d) Temperature dependence of the spectral intensity for the $\alpha$, $\beta$, $\gamma$ bands, comparing heating and cooling measurements.

[S1] T. Wang, J. Chu, J. Feng, L. Wang, X. Xu, W. Li, H. Wen, X. Liu, and G. Mu, Low temperature specific heat of 12442-type $KCa_2Fe_4As_4F_2$ single crystals, Sci. China Phys. Mech. Astron. **63**, 297412 (2020).

[S2] Z.-C. Wang, C.-Y. He, S.-Q. Wu, Z.-T. Tang, Y. Liu, A. Ablimit, C.-M. Feng, and G.-H. Cao, Superconductivity in $KCa_2Fe_4As_4F_2$ with separate double $Fe_2As_2$ layers, J. Am. Chem. Soc. **138**, 7856 (2016).

[S3] D. T. Adroja, S. J. Blundell, F. Lang, H. Luo, Z.-C. Wang, and G.-H. Cao, Observation of a neutron spin resonance in the bilayered superconductor $CsCa_2Fe_4As_4F_2$, J. Phys.: Condens. Matter **32**, 435603 (2020).

[S4] W. Hong, L. Song, B. Liu, Z. Li, Z. Zeng, Y. Li, D. Wu, Q. Sui, T. Xie, S. Danilkin, H. Ghosh, A. Ghosh, J. Hu, L. Zhao, X. Zhou, X. Qiu, S. Li, and H. Luo, Neutron spin resonance in a quasi-two-dimensional iron-based superconductor, Phys. Rev. Lett. **125**, 117002 (2020).

[S5] C. Huang, S. Duan, and W. Zhang, High-resolution time- and angle-resolved photoemission studies on quantum materials, Quantum Front. **1**, 15 (2022).

[S6] Y. Yang, Q. Wang, S. Duan, H. Wo, C. Huang, S. Wang, L. Gu, D. Qian, J. Zhao, and W. Zhang, Unusual band splitting and superconducting gap evolution with sulfur substitution in FeSe, Chin. Phys. Lett. **39**, 057302 (2022).

[S7] S. Duan, S. Wang, Y. Yang, C. Huang, L. Gu, H. Liu, and W. Zhang, A sample-position-autocorrection system with precision better than 1 $\mu$m in angle-resolved photoemission experiments, Rev. Sci. Instrum. **93**, 103905 (2022).

[S8] W. Duan, K. Chen, W. Hong, X. Chen, H. Yang, S. Li, H. Luo, and H.-H. Wen, Single-particle tunneling spectroscopy and superconducting gaps in the layered iron-based superconductor $KCa_2Fe_4As_4F_2$, Phys. Rev. B **103**, 214518 (2021).

[S9] S. Shao, F. Zhang, Z. Zhang, T. Wang, Y. Wu, Y. Tu, J. Hou, X. Hou, N. Hao, G. Mu, and L. Shan, Superconductivity and pseudogap features of an isolated FeAs layer in $KCa_2Fe_4As_4F_2$ unraveled by stm/sts, Sci. China Phys. Mech. Astron. **66**, 287412 (2023).

[S10] H. Liu, S. Duan, X. Liu, Z. Liu, S. Wang, L. Gu, J. Huang, W. Yang, J. Liu, D. Qian, Y. Guo, and W. Zhang, Fluctuated lattice-driven charge density wave far above the condensation temperature in kagome superconductor $KV_3Sb_5$, Science Bulletin **70**, 1211 (2025).

[S11] J. Bardeen, L. N. Cooper, and J. R. Schrieffer, Theory of superconductivity, Phys. Rev. **108**, 1175 (1957).

[S12] V. G. Kogan, C. Martin, and R. Prozorov, Superfluid density and specific heat within a self-consistent scheme for a two-band superconductor, Phys. Rev. B **80**, 014507 (2009).

[S13] R. Prozorov and V. G. Kogan, London penetration depth in iron-based superconductors, Rep. Prog. Phys. **74**, 124505 (2011).

[S14] G. Eilenberger, Transformation of Gorkov's equation for type II superconductors into transport-like equations, Z. Physik **214**, 195 (1968).
